# Supplementary material for: Show Me the Money: Dynamic Recommendations for Revenue Maximization
Source: arXiv:1409.0080 source file (2015-08-25)
Supplement: Supplementary file 1 [file appendix.tex]

We are grateful for the revision opportunity and would like to thank the reviewers and the meta-reviewer for their careful reading of the paper and their excellent comments. We have addressed every single comment carefully and have thoroughly revised the paper. 

\spara{Highlights of changes:} 
(1).\ We refined the writing and presentation throughout the paper, keeping in mind the reviewers' concern that \revmax uses too many parameters. In \textsection\ref{sec:revmax}, we now keep only the essential parameters needed for the core \revmax problem. Specifically, our framework and results are  orthogonal to the details of how primitive adoption probabilities are computed: the hardness remains (even when there is no saturation) and all algorithms are applicable regardless of how primitive adoption probabilities are computed. Those details are now deferred to \textsection\ref{sec:exp}. 

(2).\ We provide a justification of the assumptions made in the paper. E.g., the assumption about independent private valuations and about users being price takers are both standard in the economics literature, which we cite and explain.  

(3).\ We added a new set of experiments to demonstrate the efficiency and scalability of \GGreedy. In the process of doing so, we further improved the efficiency of the version of  \GGreedy in the original submission, by using a notion of two-level heaps (see \textsection\ref{sec:gg}). In a nutshell, our experiments show that \GGreedy easily scales to a dataset which is 2.5 times the size of Netflix, the largest public ratings dataset used in RS research  (see Figure \ref{fig:syn_time}). 

(4).\ The exact price model used in the paper is standard in economics literature, which we cite. That said, we have taken reviewer 2's suggestion seriously and 
%discuss how a random price model can be handled within our framework. Specifically, we 
added a new section (\textsection\ref{sec:discuss}) discussing how to incorporate a probabilistic price prediction model into our framework. The NP-hardness remains. On the positive side, our algorithms can still be leveraged by making use of Taylor approximation. 

(5).\ In order to make room for the new materials added to the paper, the following material was removed/suppressed:
(i).\ we replaced the complete proof of Theorem~\ref{thm:sm} with a sketch.
(ii).\ we removed the pseudo-code of \RGreedy, due to its similarity to \SGreedy (Algorithm~\ref{alg:sg}).

\eat{ 
(1).\ We further improved the efficiency of our best greedy algorithm, \GGreedy, by introducing the notion of two-level heaps. This cut the running time by approximately 50\% on Amazon and Epinions. Please refer to \textsection\ref{sec:gg} for details.

(2).\ We added a new set of experiments on larger datasets (synthetically generated) to demonstrate \GGreedy are efficient and scalable (Figure \ref{fig:syn_time}).
% and it has no problem handling data of roughly the same size as the Netflix data, which is one of the largest used in recommender systems research. 

(3).\ We added \textsection\ref{sec:discuss} to discuss the setting where fixed price values are not completely known. As suggested in Review No. 2, it is interesting to study \revmax with a random price model.
We proposed a solution framework which works for any probability distribution that prices may follow, and can be nicely integrated into current algorithms, e.g., \GGreedy.
}

%Next, we give detailed responses to each comment in the reviews.

\subsection*{Review No.\ 1 by Assigned\_Reviewer\_17}

\noindent\textit{Comment 1: The proposed dynamic adoption probability has many assumptions and parameters.}

\ipara{Response:}
\eat{The probability of a consumer adopting a product can be indeed complex, but we agree that technically the model should be clean and simple and still capture the essence of \revmax. As shown in the proof of Theorem \ref{thm:nph}, \revmax remains NP-hard even if the saturation parameter for all items are 1, which means even we do not consider saturation at all, \revmax remains challenging. 
The dynamic adoption probability consists of two parts: the primitive value, which is strategy-independent, and factors that are strategy-dependent such as competition and saturation.
The primitive part is considered as an orthogonal component (i.e., they are externally determined and are given as input).
In our refined presentation, we make this explicit and introduce it as a more abstract notion: it is anti-monotone w.r.t.\ price and different sellers may want to model it differently. Our experiments used predicted ratings and valuation distribution to estimate such values.
}
We have reorganized the presentation. In the \revmax problem definition (\textsection\ref{sec:revmax}), we only retain the crucial features, including prices, (primitive) adoption probabilities,  competition, and saturation. Saturation can be turned off or on by setting the parameter $\beta_i$ to be $1$ or $< 1$. The technical results and algorithms are unaffected by this reorganization. Specifically, the proof of NP-hardness is intact and the algorithms work regardless of {\sl how} the adoption probabilities are computed and whether saturation is present. The key intuition is that the core problem where we have item capacity constraints, display constraint, and primitive adoption probabilities together with  competition is NP-hard. This remains true regardless of whether the price model is exact or random (i.e., probabilistic). The details of how the adoption probabilities are computed are orthogonal to our framework and are deferred to \textsection\ref{sec:exp}. On the other hand, our algorithms can handle many natural additional features that may be at play in the context of revenue maximizing recommendations: user saturation from repeated recommendation, and specific ways of estimating primitive adoption probabilities, say from ratings and user valuations. 
We believe it is an intuitive and principled way to estimate, but recognize that alternative methods do exist, e.g., \cite{zhao12} (please see the discussion on this in \textsection\ref{sec:related}).
We hope that the reorganization significantly improves the clarity and positioning. 

\eat{
The key intuition is that the core problem where we have item capacity constraints, display constraint, and primitive adoption probabilities together with the notion of item categories (competition) is NP-hard. This remains true regardless even if prices are known only probabilistically. On the other hand, our algorithms can handle many natural additional features that may be at play in the context of revenue maximizing recommendations: user saturation from repeated recommendation, and specific ways of estimating primitive adoption probabilities, say from ratings and user valuations. 
We believe it is an intuitive and principled way to do it, but alternative methods do exist, e.g., \cite{zhao12} (see the discussion on this in \textsection\ref{sec:related}).
} 

\ipara{Comment 2: Datasets used in experiments are too small (5000 items for Amazon).}

\ipara{Response:}
Thank you for this comment. It inspired us to conduct scalability experiments and in the process, we ended up improving the performance of the previous version of the \GGreedy algorithm. Specifically, we have added a set of synthetic data experiments with much larger input size, to demonstrate that \GGreedy, the best of our proposed algorithms, can handle much larger datasets (\textsection\ref{sec:result}, p.11).
The running time  of the proposed algorithms is determined by \emph{the number of non-zero adoption probabilities}, i.e., the number of (user, item, time) triples for which the user has some interest in the item at that time.
In our experiments, we first ranked the items based on their predicted ratings and pick the top-$N$ for consideration (a user will only have non-zero adoption probability for those).
Under this setting, running time is directly dependent on the number of users, but  not on the number of items.
%This in turns means running time goes up as the number of users goes up.
We generated 5 synthetic datasets, with 100K--500K users.
In the largest one, there are 250 million triples ($T=5, N=100$) that \GGreedy will rank and select.
To put it in perspective, the Netflix rating data in the Netflix competition has 480K users and 100 million ratings, and is among the largest public dataset used in RS research. Our results show that the performance scales almost linearly, with \GGreedy running on the largest dataset in about 13 minutes (see Figure~\ref{fig:syn_time}). 

{\sl For Amazon}: 
\eat{We want only popular items so that there are a large number of ratings available (thus rating prediction is more accurate). We also want the users rating these items to have a certain degree of overlap.
For example, people who buy many Books on Amazon may not buy Electronics or Home Appliances on Amazon at all.
Thus, we decided to focus on a single product category.}
Obtaining real datasets which include all or even most of the features we need for our problem is hard and time consuming: we did 3-month daily crawling from Amazon to collect the dataset we used, and we did our best in order to find a way to obtain a 3-month price series from Amazon for the items in the crawled data. The reason to select popular items is that they receive enough ratings for computing predicted ratings in a {\sl reliable} manner. The reason to focus on Electronics category is that we want the sets of buyers of different items to have a certain degree of overlap. This left us with 4.2K items. 

{\sl For Epinions}: since reporting prices in reviews is optional, there were not many products that have many prices, for estimating price and valuation distributions. 
We had to filter out items with less than 10 prices (to make the number of samples reasonable), and this left us with 1.1K items.  

\emph{\sf Thus, to mitigate scalability concerns, we have used synthetic datasets as reported above.}  

\eat{
To the best of our knowledge, all public accessible Amazon data do not come with ground-truth time series of prices.
There exist price tracking website for Amazon (camelcamelcamel.com), but they only present graphical information (price trends) and do not disclose exact values.
Thus we made a three-month crawling effort to get the data.
We would be more than happy to make our Amazon dataset publicly available for research use in the future. 
}

\ipara{Revision Sought: Give more details on the assumptions and parameters of the paper to convince the readers.}

\ipara{Response:}
We have rewritten \textsection\ref{sec:intro} and \textsection\ref{sec:revmax}, where we gave a rationale for every parameter included in the framework and also cited relevant literature to support assumptions made (see also response to Comment 1 above). Specifically, competition and saturation are justified and motivated in \textsection\ref{sec:intro}, while display and capacity constraints are motivated in \textsection\ref{sec:revmaxdef}, where we also explain that the time horizon considered for recommendation strategies is short (e.g., a week) and the items considered are expensive (e.g., electronic gadgets and appliances). A user is unlikely to buy any one of such items (or items from its class) repeatedly over a short horizon. 

\ipara{Revision Sought: Please explain why only select 5000 popular items. To demonstrate the
effectiveness and efficiency of the proposed local search approximation
algorithm and those greedy heuristics, some larger data set needs to be
used.}

\ipara{Response:}
Please see the response to Comment 2.

\subsection*{Review No.\ 2 by Assigned\_Reviewer\_19}

%The weakness comment and revisions sought are closely related.

\ipara{Comment 1: The model with complete price information on all timestamps looks unrealistic.}

\ipara{Response:}
We discussed this issue at length with an economics expert. 
Complete price information (called \emph{exact price model} in the revision) corresponds to the well-known fixed-price model in economics theory.
Micro-economists have developed methodology to predict future demand and supply of a good and thus determine its price at market equilibrium (see, e.g., Ch. 17 in \cite{snyder08}).
Also, %though we cannot speak for all retailers, 
many businesses do release future pricing plans ahead of time, e.g., weekly flyers and advertisement for big sale dates like Black Friday in the US and Boxing Day in Canada. Thus, we believe this model is reasonable. 
\eat{
We also talked with economics experts at our institution (who is not involved in and had no prior knowledge of this work), who thought the fixed-price model is reasonable for our purpose.
}
That said, we  agree that \revmax with random (i.e., probabilistic) prices (see next comment) is a very appealing problem to study.
Therefore, we dedicated a new section \textsection\ref{sec:discuss} to describing how our framework can deal with this alternative price model. In both cases -- exact or random price model -- the price model is exogenous to the RS. 

\ipara{Revisions Sought: For a recommendation system in the real world, it is unlikely to have all such price information of next few hours, or new few days. It means that it is impossible for any recommendation system to schedule the target customers for expected price plans. 

To fix the problem, the key is to revise the model, with distribution assumption on prices of the products and independence between prices (probably not good as well, as the prices of competitive products could be correlated). Based on the revised model, is it possible to update the current algorithms and design the online versions, to support the online recommendations? Update the problem definition and assumptions behind the model; Design online recommendation algorithms; Re-test the experiments under online setting.} 

\ipara{Response:}
\eat{
For this suggestion, after much exploration and discussions, we decided to go for a middle-ground solution. 
} 
Firstly, as mentioned in the response to Comment 1, methodologies exist in the economics literature to predict future prices in accordance with the exact price model. Thus this assumption is not only realistic, it is standard in the economics literature. 

Secondly, we do agree that the random price model where prices are predicted to within a distribution is an appealing one and have dedicated a section (\textsection\ref{sec:discuss}) to discussing how this model can be handled in our framework. However, we have retained the exact price model in the bulk of the technical development and in the experiments. All our results and algorithms apply for both exact and random price models.  Furthermore, finding real datasets from which to learn the distribution parameters for the random price model is very challenging. E.g., the Amazon data we crawled only records one price per item per day, which is not sufficient to learn a price distribution for each time step! 

Thirdly, 
one can interpret ``online recommendation'' strictly to mean that the price of an item at time $t$ becomes available only at $t$, not before. Alternatively, we can interpret it to mean that item prices (whether exact or random) over a \emph{short time horizon} are available in advance. The former case can be easily handled using our \SGreedy algorithm to roll out recommendations for the current time $t$ once item prices for time $t$ become available. Then for every $(u,i)$ pair for which an adoption has been observed, we can set the adoption probabilities $\ap(u,i,t')$ to $0$, for $t' \in [T], t' > t$, before proceeding to make future recommendations. Thus, this is not an interesting case. 

The latter interpretation is more interesting and challenging and is what we focus on in the paper. Under that setting, we consider not only the exact price model, but also discuss %(\textsection\ref{sec:discuss}) 
how a random price model can be incorporated into our framework. 

\eat{
In the former case, we can directly use a simple adaptation of our algorithm \SGreedy, which makes recommendation decisions in chronological order. We just need to  easily devise the optimal recommendation strategy by generating recommendations for one time step at a time, using the static approach of making one-shot recommendations as in [21, 23], which make use of generalized bipartite matching. 

I.e, we formulate \revmax with random prices, and give a solution framework that can be nicely integrated into the current algorithmic framework proposed for \revmax with fixed price (e.g., \GGreedy).
They are presented in \textsection\ref{sec:discuss}.
The reason that we could not make this as our main model and run experiments is that it has been difficult to find a data source that could provide us with real-world data for estimating the distribution of price for all items in all time steps.
For example, the Amazon data we crawled only records one price per item per day, which is not sufficient.
It is also difficult to come up with a principled way to generate such synthetic datasets.
However, we believe that our solution outlined in \textsection\ref{sec:discuss} is still valuable and can be used for evaluation should a suitable dataset for random price model be discovered.
}

\subsection*{Review No.\ 3 by Assigned\_Reviewer\_5}

\ipara{Comment 1: Several related work are missing \cite{zhao12, wang13}. Comparative studies with these works are missing.}

\ipara{Response:}
Thanks for pointing out \cite{zhao12, wang13}: we have included them in related work (\textsection\ref{sec:related}).
Both of them focus on user-centric recommendation generation as classical RS papers do, and give elegant approaches for estimating the adoption probability of a user for an item at a given time.
In that sense, their contributions are orthogonal to those of our paper, as our framework can work with any method for estimating adoption probabilities. 
%The \revmax framework here could use the techniques of those papers for %estimating adoption probabilities.

However, a direct empirical comparison between \revmax and \cite{zhao12, wang13} in terms of revenue achieved, we are afraid, is ill-defined, as they do not fit naturally into each other's framework for the following two reasons.
First, the goal of our work is revenue maximization while that of \cite{zhao12, wang13} is to find the right timing for recommendation based on historical purchase interval, without any economic considerations. 
Second, our work generates strategic recommendation plan for a short time  horizon of 5-7 days (as one cannot really make a plan for longer terms, say a month or a year). In general, products will not be repeatedly purchased by a user within that time horizon (especially expensive electronic products, unlike products consumed daily such as groceries or gas). 
The data in \cite{zhao12} suggests that for an interval of 7 days, the density of purchase interval matrix is only 0.41\% ({\em cf.} Table 2 in \cite{zhao12}), which, we understand, is measured over all pairs of items.  Thus, for items directly competing with each other, such repeat purchase phenomenon will be even rarer.
To the best of our understanding, the work in \cite{zhao12, wang13} is better suited for settings with a much longer time period, as the historical purchase log should cover long term for the learned purchase intervals to be reliable and meaningful (the data in \cite{wang13} spans five years), and indeed many purchase intervals span weeks ({\em cf.} Table 4 in \cite{zhao12}).

In addition, we give the rationale for choosing the baselines we currently evaluate:
\topkrating relies only on ratings as most recommendation methods are simply just rating-based.
\topkrev ranks item using ``expected'' revenue (in a local sense), i.e., (price $\times$  primitive adoption probability), but does not take into account all other factors considered in our paper.
In a sense, it is an adaptation from \cite{chen08} of which the goal is the same as ours: maximizing revenue (profit).

%\note[Wei]{Laks, can you improve this response?}

\ipara{Comment 2:  In Section 3.1, the authors try to model user's preference, price, saturation
effect and competition of similar products separately. However, these
factors are correlated and could have varying importance for different
users/items.}

\ipara{Response:}
We agree a model which factors in possible interdependence between these features would be richer and interesting to study. We believe solving \revmax for the comparatively simpler case studied in the paper is a critical first step before studying more complex models. We mention this in future work. 

\eat{ 
The essential ingredients in our framework are linked as follows.
Revenue from each single triple in the recommendation strategy is computed by price multiplied by dynamic adoption probability (which is strategy dependent).
The latter, in a way, encapsulates and unifies the effect of saturation, competition, as well as user's uncertainly of adoption (primitive adoption probability).
} 

%\note[Wei]{Laks, can you give a strong rebuttal for it?}

\ipara{Comment 3:  In Section 3.1.2, $\beta_i$ does not depend on item $i$, hence the subscript $i$
can be removed.}

\ipara{Response:}
Our intention was to make $\beta_i$ be item-dependent, since saturation effect can vary between items. 
The same modeling was proposed and validated in \cite{dassarma12}.
We now use the subscript throughout the paper.

\ipara{Comment 4: In section 3.2, $\price(i,t)$ (the price of item) are assumed to be known in
advance (7 days)? It will be interesting to extend it to find the optimal price
to maximize the revenue.}

\ipara{Response:}
We agree this is a very interesting problem, but is very different from that of designing optimal {\sl recommendation strategies} given pricing information. For the purpose of \revmax,  
price information is considered exogenous and pricing is not the responsibility of a RS, but rather that of the sales and marketing department of the seller (see also \textsection\ref{sec:intro} and \textsection\ref{sec:revmax}). Optimal pricing is in fact one
of the central topics studied by economists and algorithmic game theoreticians \cite{agtbook, klbbook}. We include this in the future work. 

\eat{ 
We discussed the fixed-price assumption in the response to Review No. 2.
For determining the optimal price, it is indeed an interesting topic and is in fact one
of the central topics studied by economists and algorithmic game theoreticians \cite{agtbook, klbbook}.
For the purpose of \revmax, as we wrote in \textsection\ref{sec:intro} and \textsection\ref{sec:revmax},
price is considered exogenous and pricing is not the responsibility of a RS (but rather the sales and marketing department of the seller).
} 

\ipara{Comment 5: What is the error bounds for the greedy algorithms?}

\ipara{Response:}
All of the three greedy algorithms, as mentioned in the paper, are heuristic solutions.
Since the objective function of \revmax is non-monotone and submodular, and the capacity constraint
cannot be directly transformed into a matroid constraint, greedy solutions are not known to
have approximation guarantees under these conditions in the literature on submodular function optimization.
Detailed discussions on approximation of \revmax and its connection to submodularity and matroid theory are in \textsection\ref{sec:theory}.

\ipara{Comment 6(a): Experiments: There is no explanation on how to split the data for training and testing.}

\ipara{Response:}
Please note that rating prediction is the only part where training and testing apply. The core \revmax algorithms are optimization algorithms, {\em not}  learning algorithms. 
For rating prediction, we used five-fold cross validation to find the best regularization parameter, and then used it to compute the latent feature vectors for users and items in the entire rating matrix.
Please see \textsection\ref{sec:exp}.1.

\ipara{Comment 6(b): Experiments: There is no definition of the metrics revenue achieved in finite time
horizon [T]. Since the test set item is associated with timestamp, there are two possible ways to measure it.

Case 1: the order of recommended item matters. Calculate the revenue
achieved measured in different time points t and get the total revenue
achieved at different time points. For example, if an item x is recommend
to user in day 1,and item x is accepted by user in day 3, then the revenue
is not counted.

Case 2: the order of recommended item does not matters. Calculate the
revenue in the fixed time horizon. e.g. recommend item x in day 1, although
item x is accepted in day 3, it is considered a hit and the revenue is
counted.}

\ipara{Response}:
Comparing the algorithms w.r.t. actual revenue (whether Case 1 or Case 2) is more relevant to {\sl validating} the adoption probabilies, which is not a core contribution of this paper. Please note that the metric revenue that is measured in the experiments is the expected revenue, as defined in Def. \ref{def:rev}. The main problem studied in our paper is given a price model and a method for estimating adoption probabilities, design a recommendation strategy which optimizes the expected revenue. Thus, we compare all algorithms w.r.t. the objective they are trying to maximize. 

\eat{ 
The short answer is that neither Case 1 nor Case 2 captures the metric used.
Longer answer:
The objective function of \revmax on which algorithms are evaluated and compared
are defined in Definition \ref{def:rev}.
To reiterate, given any recommendation strategy, its value is the total expected revenue yielded collectively by all triples included in that strategy.
That is, for any (valid) recommendation strategy $S$ (output of some algorithm), each user-item-time triple $(u,i,t)\in S$
yields a certain amount of revenue {\em in expectation} and all of their contributions are totaled together, using the definition
of dynamic adoption probability ({\em cf.} Definition \ref{def:dap} and Example \ref{ex:dap}). 
%Consider the example given in the comment, when computing the expected revenue in that case, both the contribution of day 1 and day 3 will be calculated and counted.
When computing the expected revenue, the actual adoption action has not happened yet (and due to inherent uncertainly in adoption behaviors, it may never happen) as \revmax is the problem of designing a strategic recommendation plan for a short future horizon.
} 

\ipara{Comment 6(c): Experiments: In Figure 2, GGNo
changes when beta change. However, from Section
6.2, GGNo will not multiply the saturation term which contain beta.
It is not clear why does the GGNo
depends on beta in this case. The
expected revenue is nearly monotonic with respect to beta, which means
repeated recommendation is best among all strategies. This seems to
contradict the claim in Section 3.1.2.}

\ipara{Response:}
Firstly, please notice that the purpose of including GG-No in experiments is to examine how much revenue we will hurt by {\sl ignoring} saturation effect \emph{when it is actually present}, compared with GG which does not ignore it.
GG-No, when selecting triples and computing their marginal revenue, treats \emph{as though} $\beta_i$ is $1$ for all items $i\in I$ %(recall, $1$ means no saturation). It does so since 
as it ignores saturation. Of course, this revenue does not change with $\beta_i$, but notice the revenue computed by GG-No is clearly incorrect. It serves the purpose of GG-No picking some strategy, say $S$. Once $S$ is determined, we can compute the correct expected revenue taking saturation (which \emph{is} present) into account. This correct expected revenue will of course be affected by the value of $\beta_i$. 

Secondly, please notice that it is not up to the RS (or the seller) to {\sl set} the value of $\beta_i$ to a desired level. Rather, the saturation effects that may be present in buyers for different items determine the value of $\beta_i$, for various $i$, which may assume any (fixed) value in $[0,1]$. The expected revenue is of course highest when there is no saturation (when $\beta_i=1$) but this doesn't mean repeated recommendations are best among all strategies, since the seller doesn't get to control the saturation effects! The real intention in Figures 2 and 3 is to compare the quality of different algorithms for each given value of $\beta_i$. 

\eat{ 
Saturation discounts the dynamic adoption probability of repeated recommended items.
By Definition \ref{def:dap}, the smaller the $\beta$, the greater the discount will be.
When the input $\beta_i$'s are different (e.g., 0.2 vs. 0.8), the algorithm ought to output two different strategies.
However, one cannot directly compare these two strategies' value as they are defined w.r.t.\ different problem instances (inputs).
Thus in Figure 2 and 3, the intention is to compare the output of different algorithms in each case of $\beta_i$.
} 

\ipara{Comment 6(d): Experiments: In Figure 4, class size=1 (each item is in its own class, no competition
among class) is best for the two datasets. This seems to contradict the
competition effect in Section 3.1.2.}

\ipara{Response:}
Actually, the material in Section 3.1.2 (now Section 3.1) does not imply anything w.r.t. whether the expected revenue should increase or decrease as class size increases. Thus, there is no contradiction. That said, this comment made us investigate the possible reasons behind the observations in Figure 4. First, consider the two extremes: (a) every item in its own class and (b) all items forming one class. It is easy to see that all else being the same, the expected revenue for (b) will be less than that for (a). The reason is every item('s recommendation) interferes with every other item in case (b). Every user must receive $k\times T$ recommendations over the horizon and thus, these recomendations will have a much diminished dynamic adoption probability for (b) compared to that for (a). Let us  consider a case that is in between (a) and (b). In our experiments, for each user, $100$ items have non-zero adoption probability. Every user should receive $k \times T = 10 \times 7 = 70$ recommendations. When class size is 1, recommendations do not interfere with each other (in terms of diminishing the dynamic adoption probability). See Table 1, which shows the distribution of class sizes in the datasets, when we use the natural classes present there. In that case, there is a greater probability that recommendations to a user may interfere with each other.  This is the reason we are seeing a drop in the expected revenue when class size is $> 1$. Notice that this drop is not always guaranteed to occur: e.g., in another extreme case, if there is a large number of items and each class contains at most one item in any user's top-100 favorite items, then there should be no drop. 

\eat{ 
The revenue is higher in the case of category size = $1$ is actually intuitive according to competition effect.
When each item is in its own class, it will not compete with any others, thus for any recommended triple $(u,i,t)\in S$, only triples in the form of $(u,i,t')\in S$, $t' < t$ will result in discounting of $\dap_S(u,i,t)$.
If on the other hand, $i$ competes with a set of other items, then triples $(u,j,t')\in S$ with $t' \le t$ and $\cl{C}(j) = \cl{C}(i)$ will also impose discounting on $\dap_S(u,i,t)$, which further decreases its value and thus decreases the expected revenue.
} 

\ipara{Comment 6(e): Experiments: There is no experiments to study how the different factors such as
prices, valuations, saturation and competition among similar products
contribute to the revenue maximization.}

\ipara{Response:}
Prices are available in the real datasets we crawl (Amazon) or obtain from publicly available sources (Epinions), and we sample them to learn the valuation distribution. This has allowed us to stick to the ground-truth data as much as possible, instead of setting arbitrary values to those parameters.

We would like to point out that the effects of saturation are   demonstrated in Figure \ref{fig:BetaClass} and Figure \ref{fig:BetaNoClass}, where we vary the value of $\beta_i$ and compare algorithms in each case.
Competition is also studied in Figure \ref{fig:BetaClass} and Figure \ref{fig:BetaNoClass}. In one case we use ground-truth product categories to classify items that compete, and in the other, we put each item into its own category and hence study the effect of there being no competition.
The overall trend of the performance of various algorithm is consistent in those situations. 

We agree it would be interesting to synthetically assign various values for these parameters and study their effect on the expected revenue achieved by the various algorithms. Unfortunately, space limitations prevent us from including such studies. As such, we have had to remove a fair bit of material in order to make room for the new material we have had to add to the paper.
